# Supplementary material for: A scalable exponential-DG approach for nonlinear conservation laws: with application to Burger and Euler equations
Source: arXiv:2011.01316 source file (2021-04-17)
Supplement: Supplementary file 1 [file AppendixJacobian.tex]

\renewcommand{\un}{{\unm}}
\appendix

\section{Flux Jacobian of Euler equations}
\seclab{AppendixJacobian}

For the completeness, we summarize flux Jacobian of Euler equations in two- and three-dimensions.
Details can be found in \cite{masatsuka2013like}. 

\subsection{Two-dimensional Euler equation}
We consider the two-dimensional Euler equations in a component form, 
\begin{subequations}
\eqnlab{gov-euler2d}
\begin{align}
  \dd{\rho}{t}
    + \dd{}{x}\LRp{\rho u} 
    + \dd{}{y}\LRp{\rho v} &= 0,\\
  \dd{\rho u }{t} 
    + \dd{}{x}\LRp{\rho u u + \pres}
    + \dd{}{y}\LRp{\rho v u }&= 0,\\
  \dd{\rho v }{t} 
    + \dd{}{x}\LRp{\rho u v }
    + \dd{}{y}\LRp{\rho v v + \pres}&= 0,\\    
  \dd{\rho E}{t} 
    + \dd{}{x}\LRp{\rho u H }
    + \dd{}{y}\LRp{\rho v H }&= 0.
\end{align}
\end{subequations}

The flux Jacobian along $x$-direction is defined as
\begin{align*}
%\eqnlab{euler2d-fluxJacobian-x}
  A_x(q) 
  &:= \LRp{\dd{F_x(q)}{q}} \\
  &= 
  \begin{pmatrix}
    0 & 1 & 0 & 0\\
    \LRp{\frac{\gamma-1}{2}}\norm{\ub}^2 -u^2 
    & (3-\gamma)u & (1-\gamma)v & (\gamma-1)\\
    -uv  & v & u & 0 \\
    \LRp{\LRp{\frac{\gamma-1}{2}} \norm{\ub}^2 - H}u
    & H + (1-\gamma)u^2 & (1-\gamma)u v & \gamma u
  \end{pmatrix}.
\end{align*}
The flux Jacobian along $y$-direction is denoted by 
\begin{align*}
%\eqnlab{euler2d-fluxJacobian-y}
  A_y(q) 
   &:= \LRp{\dd{F_y(q)}{q}} \\
   & = 
  \begin{pmatrix}
    0 & 0 & 1 & 0\\
    -uv  & v & u & 0 \\
    \LRp{\frac{\gamma-1}{2}}\norm{\ub}^2 -v^2 
    & (1-\gamma)u & (3-\gamma)v & (\gamma-1)\\
    \LRp{\LRp{\frac{\gamma-1}{2}} \norm{\ub}^2 - H}v
    & (1-\gamma)u v  & H + (1-\gamma)v^2 & \gamma v
  \end{pmatrix}.
\end{align*}
The normal flux Jacobian reads
\begin{align*}
%\eqnlab{euler2d-fluxJacobian-normal}
A(q) &:= \nx A_x (q) + \ny A_y(q) \\
  & = 
  \begin{pmatrix}
    0 & \nx & \ny & 0\\
    \phi \nx - u\un
    & u\nx -\gammam u \nx + \un
    & u\ny -\gammam v \nx  & \gammam \nx \\
    \phi \ny - v\un
    & v\nx -\gammam u \ny  
    & v\ny -\gammam v \ny + \un  & \gammam \ny \\
    \LRp{\phi - H}\un
    & H\nx - \gammam u \un  
    & H\ny - \gammam v \un & \gamma \un
  \end{pmatrix}.
\end{align*}
where $\phi:=\LRp{\frac{\gamma-1}{2}} \norm{\ub}^2$ and $\gammam:=\gamma-1$. 

The eigenvalues and eigenvectors of normal flux Jacobian, $A=R\Lambda R^{-1}$ are
\begin{align*}
  \Lambda = 
  \begin{pmatrix}
   \un - a & 0 & 0 & 0 \\
   0 & \un & 0 & 0 \\
   0 & 0 & \un & 0 \\
   0 & 0 & 0 & \un + a
  \end{pmatrix},
\end{align*}
\begin{align*}
  R = 
  \begin{pmatrix}
   1 & 1 & 0 & 1\\
   u - a \nx & u & \tx & u + a \nx \\
   v - a \ny & v & \ty & v + a \ny \\
   H - a \un & \half\norm{\ub}^2 & u_t & H + a \un
  \end{pmatrix}
\end{align*}
and
\begin{align*}
    R^{-1} = 
  \begin{pmatrix}
   \half\LRp{\half\mm\norm{\ub}^2 + \frac{\un}{a} }
   & -\half \LRp{\mm u + \frac{\nx}{a} } 
   & -\half \LRp{\mm v + \frac{\ny}{a} }
   & \half\mm \\
   1 - \half\mm \norm{\ub}^2 & \mm u & \mm v & - \mm \\
   -u_t & \tx & \ty & 0 \\
   \half\LRp{\half \mm \norm{\ub}^2 - \frac{\un}{a}}
   & -\half\LRp{\mm u - \frac{\nx}{a}} 
   & -\half\LRp{\mm v - \frac{\ny}{a}} & \half \mm 
  \end{pmatrix}.
\end{align*}

\subsection{Three-dimensional Euler equation}

Consider the three-dimensional Euler equations in a component form, 
\begin{subequations}
\eqnlab{gov-euler3d}
\begin{align}
  \dd{\rho}{t}
    + \dd{}{x}\LRp{\rho u} 
    + \dd{}{y}\LRp{\rho v}
    + \dd{}{z}\LRp{\rho w}&= 0,\\
  \dd{\rho u }{t} 
    + \dd{}{x}\LRp{\rho u u + \pres}
    + \dd{}{y}\LRp{\rho v u }
    + \dd{}{z}\LRp{\rho w u }&= 0,\\
  \dd{\rho v }{t} 
    + \dd{}{x}\LRp{\rho u v }
    + \dd{}{y}\LRp{\rho v v + \pres}
    + \dd{}{z}\LRp{\rho w v }&= 0,\\    
  \dd{\rho w }{t} 
    + \dd{}{x}\LRp{\rho u w }
    + \dd{}{y}\LRp{\rho v w }
    + \dd{}{z}\LRp{\rho w w + \pres}&= 0,\\    
  \dd{\rho E}{t} 
    + \dd{}{x}\LRp{\rho u H }
    + \dd{}{y}\LRp{\rho v H }
    + \dd{}{z}\LRp{\rho w H }&= 0.
\end{align}
\end{subequations}

The flux Jacobians for Euler equations along $x,y,z$ direction and normal flux Jacobian, $A:=\nx A_x (q) + \ny A_y(q) + \nz A_z(q)$, are definfed as follows: 
\begin{align*}
%\eqnlab{euler3d-fluxJacobian-x}
  A_x
  &:=
  \begin{pmatrix}
    0 & 1 & 0 & 0 & 0\\
    \LRp{\frac{\gamma-1}{2}}\norm{\ub}^2 -u^2 
    & (3-\gamma)u & (1-\gamma)v & (1-\gamma)w &  (\gamma-1)\\
    -uv  & v & u & 0 & 0 \\
    -uw  & w & 0 & u & 0 \\
    \LRp{\LRp{\frac{\gamma-1}{2}} \norm{\ub}^2 - H}u
    & H + (1-\gamma)u^2 & (1-\gamma)u v & (1-\gamma)u w & \gamma u
  \end{pmatrix}, 
\end{align*}
\begin{align*}
%\eqnlab{euler3d-fluxJacobian-y}
  A_y 
   &:= 
  \begin{pmatrix}
    0 & 0 & 1 & 0 & 0 \\
    -v u  & v & u & 0 & 0 \\
    \LRp{\frac{\gamma-1}{2}}\norm{\ub}^2 -v^2 
    & (1-\gamma)u & (3-\gamma)v & (1-\gamma) w & (\gamma-1)\\
    -v w  & 0 & w & v & 0 \\
    \LRp{\LRp{\frac{\gamma-1}{2}} \norm{\ub}^2 - H}v
    & (1-\gamma)v u  & H + (1-\gamma)v^2 & (1-\gamma)v w & \gamma v
  \end{pmatrix},
\end{align*}
\begin{align*}
%\eqnlab{euler3d-fluxJacobian-z}
  A_z 
   &:= 
  \begin{pmatrix}
    0 & 0 & 0 & 1 & 0 \\
    -w u  & w & 0 & u & 0 \\
    -w v  & 0 & w & v & 0 \\
    \LRp{\frac{\gamma-1}{2}}\norm{\ub}^2 -w^2 
    & (1-\gamma)u & (1-\gamma)v & (3-\gamma) w & (\gamma-1)\\
    \LRp{\LRp{\frac{\gamma-1}{2}} \norm{\ub}^2 - H}w
    & (1-\gamma)w u  & (1-\gamma)w v & H+(1-\gamma)w^2 & \gamma w
  \end{pmatrix},
\end{align*}
and 
\begin{align*}
%\eqnlab{euler3d-fluxJacobian-normal}
A = 
  \begin{pmatrix}
    0 & \nx & \ny & \nz & 0\\
    \phi \nx - u\un
    & u\nx - \gammam u \nx + \un
    & u\ny - \gammam v \nx  
    & u\nz - \gammam w \nx  
    & \gammam \nx \\
    \phi \ny - v\un
    & v\nx - \gammam u \ny  
    & v\ny - \gammam v \ny + \un
    & v\nz - \gammam w \ny 
    & \gammam \ny \\
    \phi \nz - w\un
    & w\nx - \gammam u \nz  
    & w\ny - \gammam v \nz  
    & w\nz - \gammam w \nz + \un 
    & \gammam \nz \\    
    \LRp{\phi - H}\un
    & H\nx - \gammam u \un  
    & H\ny - \gammam v \un 
    & H\nz - \gammam w \un 
    & \gamma \un
  \end{pmatrix}
\end{align*}
where $\phi:=\LRp{\frac{\gamma-1}{2}} \norm{\ub}^2$ and $\gammam:=\gamma-1$. 

The eigenvalues and eigenvectors of $A=R\Lambda R^{-1}$ reads
\begin{align*}
  \Lambda = 
  \begin{pmatrix}
   \un - a & 0 & 0 & 0 & 0 \\
   0 & \un & 0 & 0 & 0 \\
   0 & 0 & \un + a & 0 & 0 \\
   0 & 0 & 0 & \un & 0 \\
   0 & 0 & 0 & 0 & \un 
  \end{pmatrix},
\end{align*}
\begin{align*}
  R = 
  \begin{pmatrix}
   1 & 1 & 1 & 0 & 0 \\
   u - a \nx & u &  u + a \nx & \tx & \sx \\
   v - a \ny & v &  v + a \ny & \ty & \sy \\
   w - a \nz & w &  v + a \ny & \tz & \sz \\
   H - a \un & \half\norm{\ub}^2 & H + a \un 
   & u_t & u_s 
  \end{pmatrix}
\end{align*}
and
\begin{align*}
    R^{-1} = 
  \begin{pmatrix}
   \frac{\gammam}{4}M^2 + \frac{\un}{2a}
   & -\frac{\gammam u}{2a^2} - \frac{\nx}{2a}
   & -\frac{\gammam v}{2a^2} - \frac{\ny}{2a}
   & -\frac{\gammam w}{2a^2} - \frac{\nz}{2a}
   & \frac{\gammam}{2a^2} \\
   1 - \frac{\gammam}{2}M^2 
   & \frac{\gammam u}{a^2} 
   & \frac{\gammam v}{a^2} 
   & \frac{\gammam w}{a^2} 
   & - \frac{\gammam }{a^2} \\
   \frac{\gammam}{4}M^2 - \frac{\un}{2a}
   & -\frac{\gammam u}{2a^2} + \frac{\nx}{2a}
   & -\frac{\gammam v}{2a^2} + \frac{\ny}{2a}
   & -\frac{\gammam w}{2a^2} + \frac{\nz}{2a}
   & \frac{\gammam}{2a^2} \\
   - u_t & \tx & \ty & \tz & 0 \\
   - u_s & \sx & \sy & \sz & 0
  \end{pmatrix}
\end{align*} 
where $M^2:= \frac{\norm{\ub}^2}{a^2}$; ${\bf t}$ and ${\bf s}$ are tangent vectors such that ${\bf s}\times {\bf t} = \nb $, ${\bf t}\times {\bf n} = {\bf s} $ and ${\bf n}\times {\bf s} = {\bf t} $; $u_t= \ub \cdot {\bf t}$ and $u_s = \ub \cdot {\bf s}$. 
